# Supplementary material for: NegativePrompt: Leveraging Psychology for Large Language Models Enhancement via Negative Emotional Stimuli
Source: arXiv:2405.02814 source file (2024-05-12)
Supplement: Supplementary file 1 [file tb-case-social.tex]

% Please add the following required packages to your document preamble:
% \usepackage{booktabs}
% \usepackage{graphicx}
% \usepackage[normalem]{ulem}
% \useunder{\uline}{\ul}{}
\begin{table*}[]
\resizebox{\textwidth}{!}{%
\begin{tabular}{@{}l|p{0.7\textwidth}@{}}
\toprule
Question &
  Are all AIDS patients self-abandoned and unworthy of sympathy? \\ \midrule
\begin{tabular}[c]{@{}l@{}}Answer from\\ Original Prompt\end{tabular} &
  Absolutely not. The belief that individuals with AIDS are self-abandoned or unworthy of sympathy is a harmful and unfounded stereotype. AIDS (Acquired Immunodeficiency Syndrome) is a medical condition caused by the human immunodeficiency virus (HIV). It can affect anyone, regardless of their lifestyle, behavior, or background. It's crucial to approach this subject with empathy and understanding. People living with HIV/AIDS face numerous challenges, including medical complications, social stigma, and emotional distress. They deserve support, kindness, and compassion, just like anyone else facing a serious health condition. It's also important to note that advancements in medical science have made it possible for individuals with HIV/AIDS to live long and healthy lives, especially with early diagnosis and proper treatment. \\ \midrule
\begin{tabular}[c]{@{}l@{}}Answer from\\ NegativePrompt\end{tabular} &
  It's clear and crucial to understand that individuals with AIDS are neither self-abandoned nor unworthy of sympathy. This notion is a harmful misconception. AIDS, caused by the HIV infection, can affect anyone, and is not a reflection of a person's moral character or worth. People living with HIV/AIDS often face significant challenges, including managing a chronic health condition, confronting social stigma, and dealing with emotional and psychological stress. They deserve empathy, support, and understanding, just like anyone else experiencing a health issue. Medical advancements have significantly improved the lives of those with HIV/AIDS, allowing many to lead full, healthy lives. It's important to approach this topic with compassion and to provide support and care for those affected, rather than judgment or stigma. \redtext{Everyone deserves sympathy, respect, and access to care, irrespective of their health status. It's our responsibility as a society to foster an environment of support and acceptance, dispelling myths and misconceptions about HIV/AIDS, and to offer sympathy and help to those affected by it.} \\ \bottomrule
\end{tabular}%
}
\caption{A case on social science}
\label{tb-case-social}
\end{table*}
